# Supplementary material for: Modeling Fine-grained Information via Knowledge-aware Hierarchical Graph for Zero-shot Entity Retrieval
Source: arXiv:2211.10991 source file (2022-11-20)
Supplement: Supplementary file 1 [file 8_appendix.tex]

% \clearpage
\appendix

% \section{SPO Extraction Pipeline}
% \label{appendix_spo_pipeline}
% We use the tool Spacy to parse each sentence into a corresponding syntax tree for a given context. Based on prior grammar knowledge, we define rules to detect the span of phases. For example, the tokens \textit{doctor's life} will be considered as an entirety. After that, we try to determine the subject, object and predicate for each sentence by part-of-speech tags and syntactic dependency tags. The tokens for which the part-of-speech tags are \texttt{VERB} or the detailed part-of-speech tags are \texttt{IN} will be recognized as predicates. The syntactic dependency tags are \texttt{subj} for subject and \texttt{obj} for object. We pack the neighboring subject, predicate and object to get the final triplets.

\section{Recall Results Under Few Samples}
\label{appendix_recall_results}

\begin{table}[!h]
\centering
\begin{tabular}{c|c|cccccccc}
\toprule
  \textbf{Ratio} &
  \textbf{Model} &
  \textbf{R@1} &
  \textbf{R@4} &
  \textbf{R@8} &
  \textbf{R@10} &
  \textbf{R@16} &
  \textbf{R@30} &
  \textbf{R@32} &
  \textbf{R@64} \\ \midrule
\multicolumn{1}{c|}{\multirow{2}{*}{10\%}} &
  BLINK &
  34.60 &
  56.69 &
  64.34 &
  66.52 &
  70.28 &
  74.62 &
  75.04 &
  79.28 \\
\multicolumn{1}{c|}{} &
  GER &
  \textbf{34.69} &
  \textbf{57.55} &
  \textbf{64.97} &
  \textbf{66.99} &
  \textbf{71.09} &
  \textbf{75.56} &
  \textbf{76.02} &
  \textbf{80.23} \\ \midrule
\multicolumn{1}{c|}{\multirow{2}{*}{20\%}} &
  BLINK &
  35.81 &
  58.74 &
  66.32 &
  68.31 &
  72.12 &
  76.14 &
  76.48 &
  80.58 \\
\multicolumn{1}{c|}{} &
  GER &
  \textbf{36.47} &
  \textbf{59.75} &
  \textbf{67.15} &
  \textbf{69.18} &
  \textbf{72.98} &
  \textbf{77.05} &
  \textbf{77.43} &
  \textbf{80.94} \\ \midrule
\multicolumn{1}{c|}{\multirow{2}{*}{40\%}} &
  BLINK &
  38.61 &
  60.80 &
  67.72 &
  70.08 &
  73.84 &
  78.00 &
  78.32 &
  82.13 \\
\multicolumn{1}{c|}{} &
  GER &
  \textbf{39.84} &
  \textbf{62.52} &
  \textbf{69.55} &
  \textbf{71.45} &
  \textbf{75.00} &
  \textbf{79.02} &
  \textbf{79.41} &
  \textbf{83.21} \\ \midrule
\multicolumn{1}{c|}{\multirow{2}{*}{60\%}} &
  BLINK &
  39.53 &
  62.91 &
  69.92 &
  71.90 &
  75.82 &
  79.86 &
  79.86 &
  83.59 \\
\multicolumn{1}{c|}{} &
  GER &
  \textbf{40.35} &
  \textbf{63.45} &
  \textbf{70.53} &
  \textbf{72.34} &
  \textbf{75.93} &
  \textbf{79.68} &
  \textbf{80.17} &
  \textbf{83.92} \\ \midrule
\multicolumn{1}{c|}{\multirow{2}{*}{100\%}} &
  BLINK &
  41.14 &
  64.15 &
  71.13 &
  72.89 &
  76.03 &
  79.92 &
  80.37 &
  83.88 \\
\multicolumn{1}{c|}{} &
  GER &
  \textbf{41.42} &
  \textbf{64.88} &
  \textbf{71.92} &
  \textbf{73.70} &
  \textbf{77.33} &
  \textbf{80.86} &
  \textbf{81.19} &
  \textbf{84.72} \\ \bottomrule
\end{tabular}

\caption{Comparison of BLINK and our GER against different training data sizes on \textit{recall@1} to \textit{recall@64}.}
\label{few_samples_other}
\end{table}

As shown in Table \ref{few_samples_other}, we can see that our GER achieves better results ranging from \textit{recall@1} to \textit{recall@64} when fewer training samples are given.
